# Supplementary material for: Causal graph fusion across incomplete cohorts and causal steering of tabular foundation models
Source: arXiv:2611.09400 source file (2026-11-06)
Supplement: Supplementary file 1 [file supplement.tex]

% Standalone Supplementary Information.
% Shares the SI body with the combined manuscript via \input{si-body}.
% Cross-references to the main text resolve through xr-hyper (reads main.aux),
% so compile main.tex first, then: pdflatex supplement; bibtex supplement; pdflatex x2.
\PassOptionsToPackage{table}{xcolor}
\documentclass[fleqn,10pt]{article}
\usepackage[utf8]{inputenc}
\usepackage[T1]{fontenc}
\usepackage[margin=2.2cm]{geometry}
\usepackage{booktabs}
\usepackage{multirow}
\usepackage{tabularx}
\usepackage{makecell}
\usepackage{array}
\usepackage{amsmath}
\usepackage{amssymb}
\usepackage{amsthm}
\usepackage{graphicx}
\usepackage{longtable}
\usepackage{tikz}
\usepackage{caption}
\usepackage{placeins}
\usepackage{algorithm}
\usepackage{algpseudocode}
\usepackage[table]{xcolor}
\usepackage[normalem]{ulem}
\newtheorem{theorem}{Theorem}
\newtheorem{lemma}{Lemma}
\usepackage{hyperref}
\usepackage{xr-hyper}
\externaldocument{main}    % resolve \ref to main-text figures/sections
\graphicspath{{figures/}{./}}
\renewcommand{\thesection}{S\arabic{section}}
\captionsetup{labelfont=bf}
\title{\vspace{-2em}\textbf{Supplementary Information}\\[0.3em]
\large Causal graph fusion across incomplete cohorts: predicting secondary complications after spinal cord injury}
\date{}
\begin{document}
\maketitle
\vspace{-1.5em}
\noindent This Supplementary Information accompanies the main manuscript; equation, figure, and section references of the form ``Figure~1'', ``Table~1'', etc.\ without an ``S'' prefix point to the main text.
\input{si-body}
\bibliographystyle{plain}
\bibliography{references}
\end{document}
